# Supplementary material for: Stochastic BIQA: Median Randomized Smoothing for Certified Blind Image Quality Assessment
Source: arXiv:2411.12575 source file (2024-11-19)
Supplement: Supplementary file 1 [file X_suppl.tex]

\clearpage
\setcounter{page}{1}
\maketitlesupplementary

\subsection{Choosing parameters for the denoiser training}

In this experiment, we used the KonCept quality metric as the base metric for the Median Smoothing and set $\sigma$ to 0.12, $\epsilon$ to 0.12, and $N\_SAMPLES$ to 2000. 

\textbf{Coefficients in the loss function.} Batch size was equal to 5. We fixed all parameters except coefficients in the loss function and compared the performance of the trained denoisers based on changes in these parameters. Equation \ref{eq:appendix_loss} presents the overall overview of the used loss function.

\begin{equation}
\begin{array}{cc}
L = MSE_{loss} + C_r * RANK_{loss} + C_t * TARG_{loss}
\end{array}
\label{eq:appendix_loss}
\end{equation}

We conducted experiments with the following grids of parameters: $C_t$ = [1, 10, 100, 1000, 10000],  $C_r$ = [1, 10, 100, 1000, 10000].

Heatmap \ref{fig:loss_coeffs} shows the experiment results. Each element in the heatmap corresponds to some denoiser, trained with $\sigma = 0.12$ on 8,000 images from the KonIQ dataset. The training was performed as the finetuning from the weights of denoiser trained only for $MSE_{loss}$ component. Each finetuning was performed for 50 epochs with $lr=0.0001$. The weights best on validation data (1,000 images from the KonIQ, different from the training set) were selected for further testing. The results in the heatmap were calculated on 1400 test images from the KonIQ dataset (different from the training and validation sets). We wish to have the denoiser, implemented in the Median Smoothing pipeline, provide high correlations of the defended metric scores with subjective scores while maintaining a lower certified delta. The certified delta was averaged across all tested images. We determined that the optimal values of the coefficients are $C_r = 1$ and $C_t = 1000$. These values provide the best balance between correlation with subjective scores and the certified delta during the experiments.

\begin{figure*}[ht]
\begin{center}
\centerline{\includegraphics[width=\linewidth]{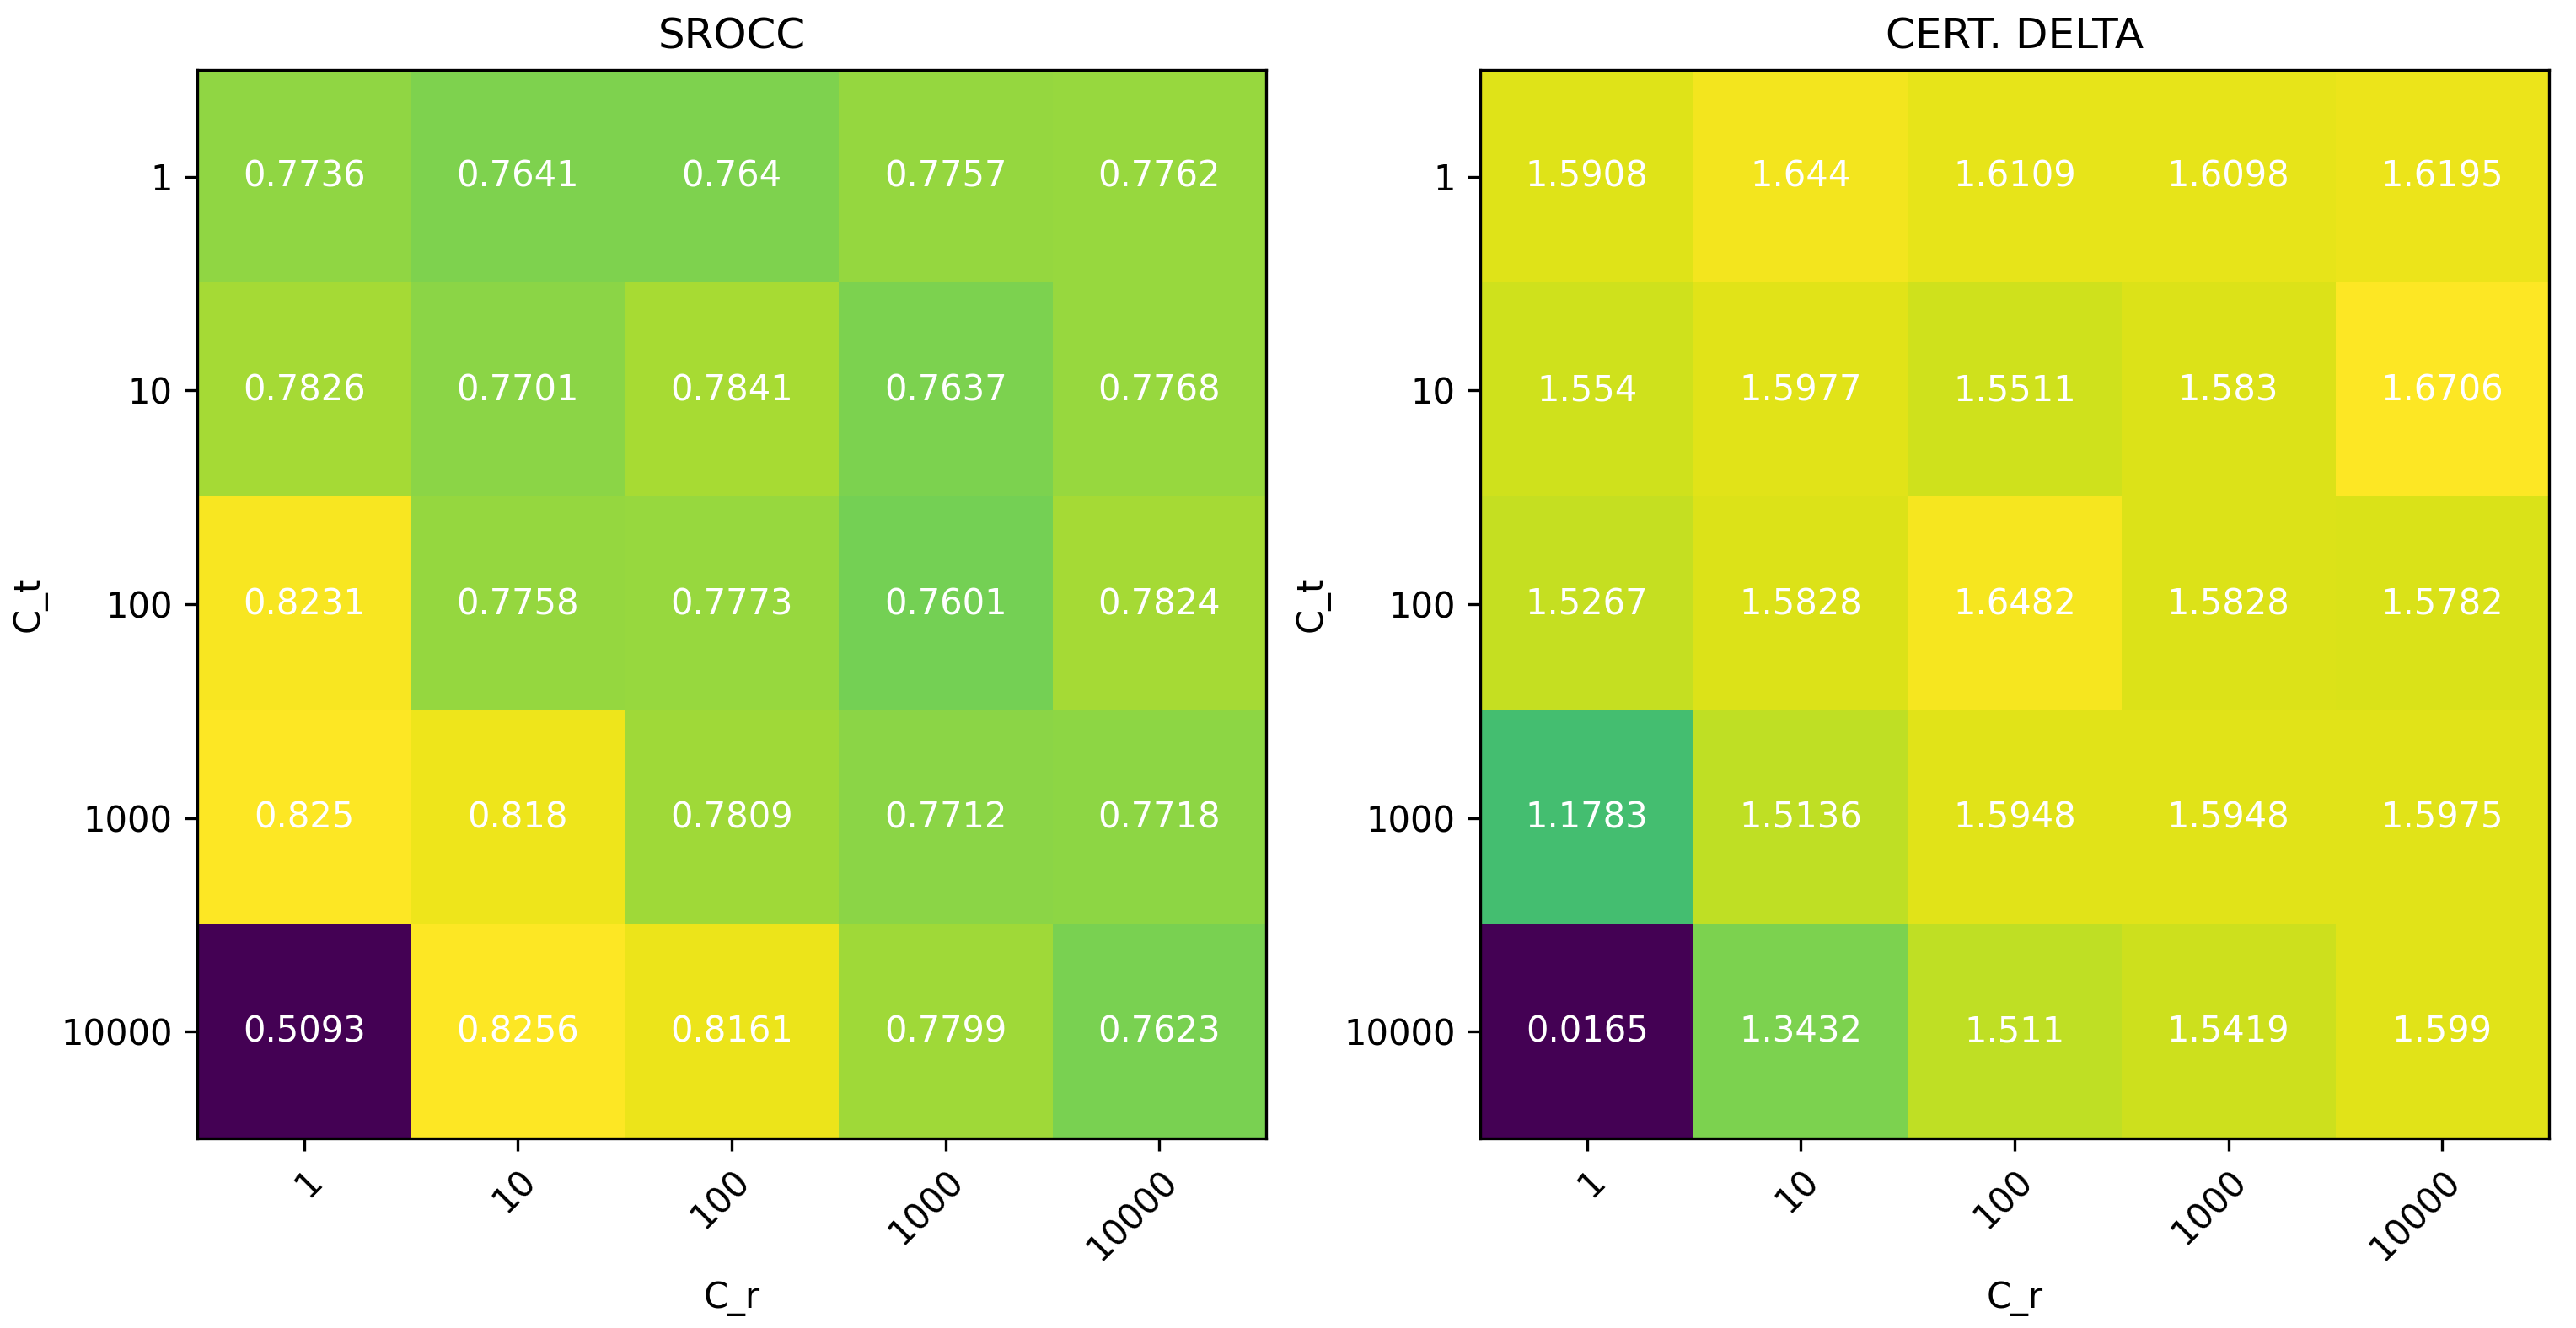}}
\caption{SROCC $\uparrow$ and Certified Delta $\downarrow$ for different loss function coefficients. The best loss function coefficients are $C_r = 1$ and $C_t = 1000$}
\label{fig:loss_coeffs}
\end{center}
\end{figure*}

\textbf{The batch size.} In this experiment, we used the best-performing loss function from the previous experiment and trained the denoisers with varying batch sizes. We used the same base metric and $\sigma$ and $\epsilon$ parameters. We used the following values for batch sizes: [3, 5, 7, 10, 15, 20]. In all experiments, the number of epochs was set to 50. Figures \ref{fig:batch_size_srocc} and \ref{fig:batch_size_delta} presents the results of the experiments, they were calculated on the test data. From the Figure \ref{fig:batch_size_srocc} we can see that greater batch size provides better overall SROCC, but it requires more RAM. Also, Figure \ref{fig:batch_size_delta} shows that for greater batch size the resulting averaged certified delta on test data is higher, we assume that this is because the overall number of training iterations for greater batch size is lower. To achieve the same certified delta for greater batch size, we need to perform training using more epochs, which is time-consuming. For practical reasons, including time and memory constraints, we used a batch size equal to 15. This batch size allows us to achieve high correlations and a good certified delta on the test data.

\begin{figure*}[ht]
\begin{center}
\centerline{\includegraphics[width=4.5in]{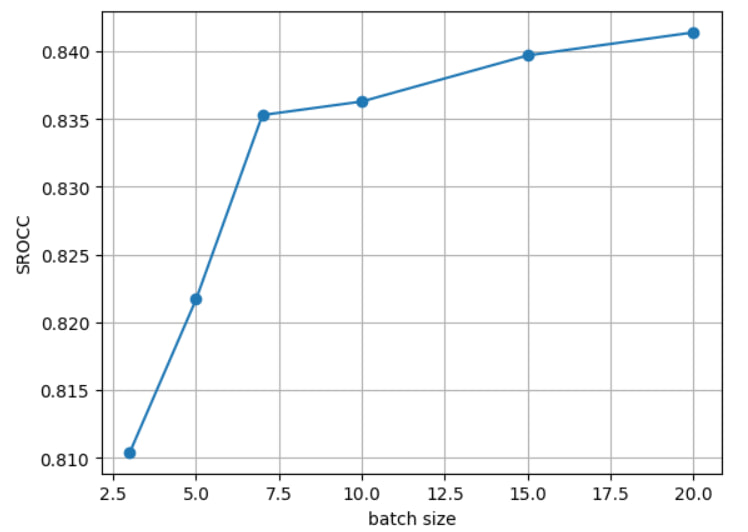}}
\caption{batch size srocc.jpg}
\label{fig:batch_size_srocc}
\end{center}
\end{figure*}

\begin{figure*}[ht]
\begin{center}
\centerline{\includegraphics[width=4.5in]{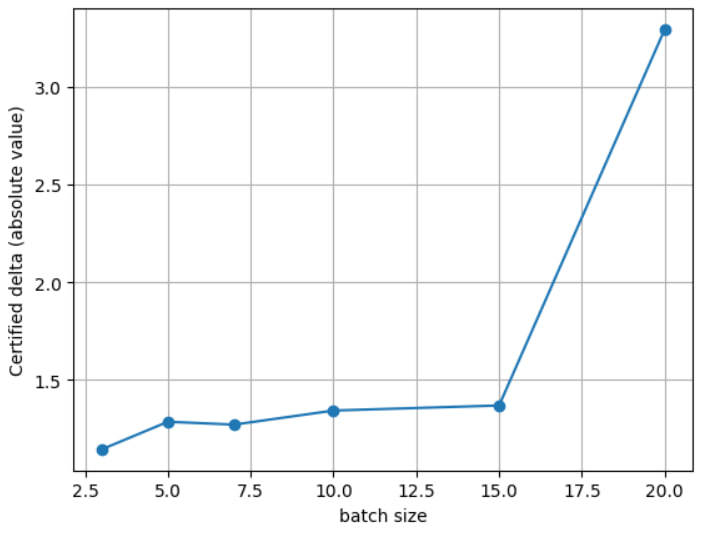}}
\caption{batch size delta.jpg}
\label{fig:batch_size_delta}
\end{center}
\end{figure*}

\subsection{Choosing presets for attacks}
For median smoothing, we cannot arbitrarily choose the values of $\epsilon$ and $\sigma$, as a high $\frac{\epsilon}{\sigma}$ ratio results in upper and lower bounds that are too far from the center. Figure 1 shows the dependency between the number of samples needed to compute certified delta and the $\frac{\epsilon}{\sigma}$ ratio. We observe that when $\epsilon \ge 3 \sigma$, more than 10,000 samples are required, making this approach extremely time-consuming. Since we aim to use around 2,000 samples, we do not consider $\frac{\epsilon}{\sigma}$ ratios greater than 2.

%\begin{table}[htb]
%\caption{Chosen parameters.}
%\label{tab:related-works}
%\begin{center}
%\begin{small}
%\begin{tabular}{lccc}
%\toprule
%Use case & $\epsilon$ & $\sigma$ & N samples \\
%\midrule
%Weak attack & 0.05 & 0.12 & 2,000 \\
%Strong attack & 0.72 & 0.36 & 2,000 \\
%\bottomrule
%\end{tabular}
%\end{small}
%\end{center}
%\end{table}

\begin{figure*}[ht]
\begin{center}
\centerline{\includegraphics[width=6.0cm]{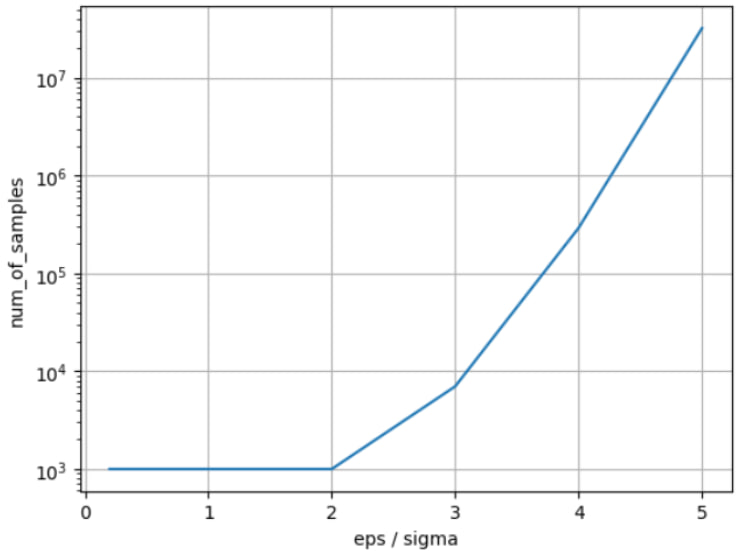}}
\caption{eps and sigma}
\label{fig:eps_sigma}
\end{center}
\end{figure*}

This section presents the experiments that led to selecting the parameters for attack strength. The target NR-IQA model used in this experiment was KonCept. We conducted additional experiments with the following parameter grids: $\sigma$ = [0.12, 0.18, 0.24, 0.3, 0.36, 0.42],  $\epsilon$ = [0.06, 0.12, 0.24, 0.36, 0.42, 0.5, 0.64, 0.72]. The number of samples for smoothing was set to 2000. Heatmap 1 shows the Spearman correlation coefficients (SROCC) between the scores produced by MS-defended, DMS-defended, and DMS-IQA-defended (ours) versions of KonCept and the subjective scores (MOS) on 1,359 images from the KonIQ dataset (test set). Heatmap 2 shows the ranges of certified deltas for the same defended variations of the model.
These heatmaps show that changes in $\epsilon$ for a fixed $\sigma$ do not significantly affect the SROCC. However, the range of certified deltas changes dramatically as $\epsilon$ increases, indicating that the robustness of the certified guarantees is highly sensitive to the choice of $\epsilon$.

We wish to have a defended model, such that the drop in correlations with subjective scores decreases no more than 10\% and the certified delta is at least 30\% larger than the adversarial gain. Based on these assumptions, we chose the following parameters for attack presets: weak use case ($\sigma$ = 0.12, $\epsilon$ = 0.06) and strong use case ($\sigma$ = 0.18, $\epsilon$ = 0.36). Here, $\epsilon$ represents the $l_2$-norm of the adversarial examples, which is used to test the target NR-IQA model. The method guarantees a certified prediction for any adversarial example with an $l_2$-norm less than $\epsilon$.

\subsection{Methods' comparison at different smoothing parameters ($\epsilon, \sigma$)}

This section shows that the proposed method is superior among others for any noise level $\sigma$ and any $l_2$ norm restriction $\epsilon$. We generated 100 adversarial examples for each $l_2$ norm using the algorithm described in Section X. The first heatmap in Figure \ref{fig:heatmap_cdelta} shows the adversarial gain for these examples. We can see that with an increase in the $l_2$ norm, adversarial gain also increases since stronger perturbation, in this case, is allowed.

The SROCC of the undefended KonCept metric on Koniq-10K is 0.8576.

\begin{figure*}[ht]
\begin{center}
\centerline{\includegraphics[width=\linewidth]{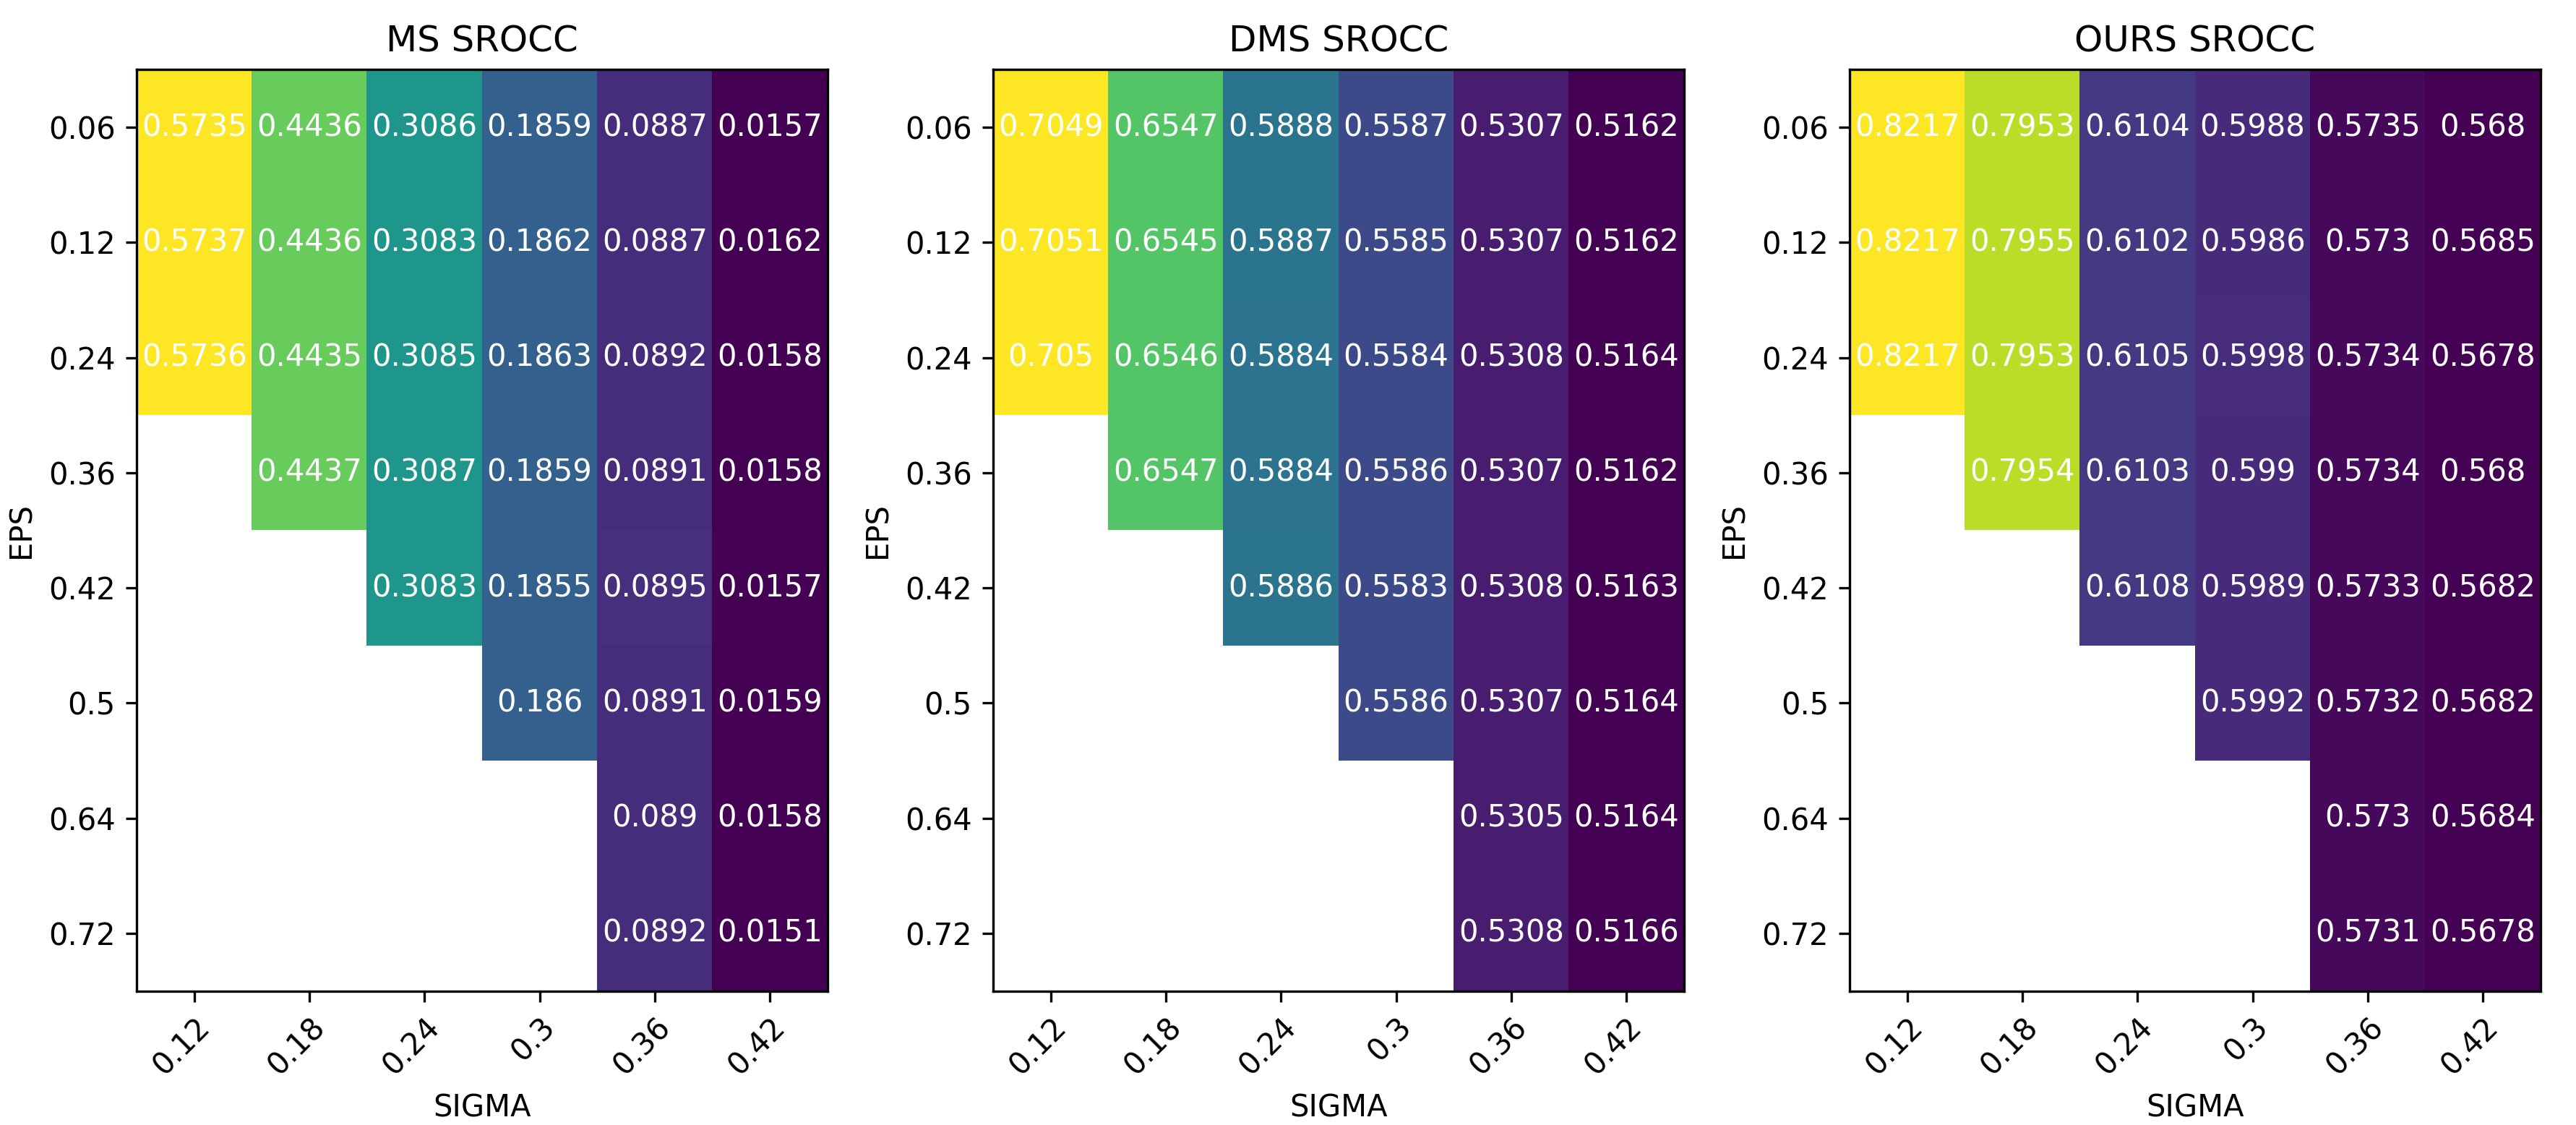}}
\caption{SROCC $\uparrow$}
\label{fig:heatmap_srocc}
\end{center}
\end{figure*}

\begin{figure*}[ht]
\begin{center}
\centerline{\includegraphics[width=\linewidth]{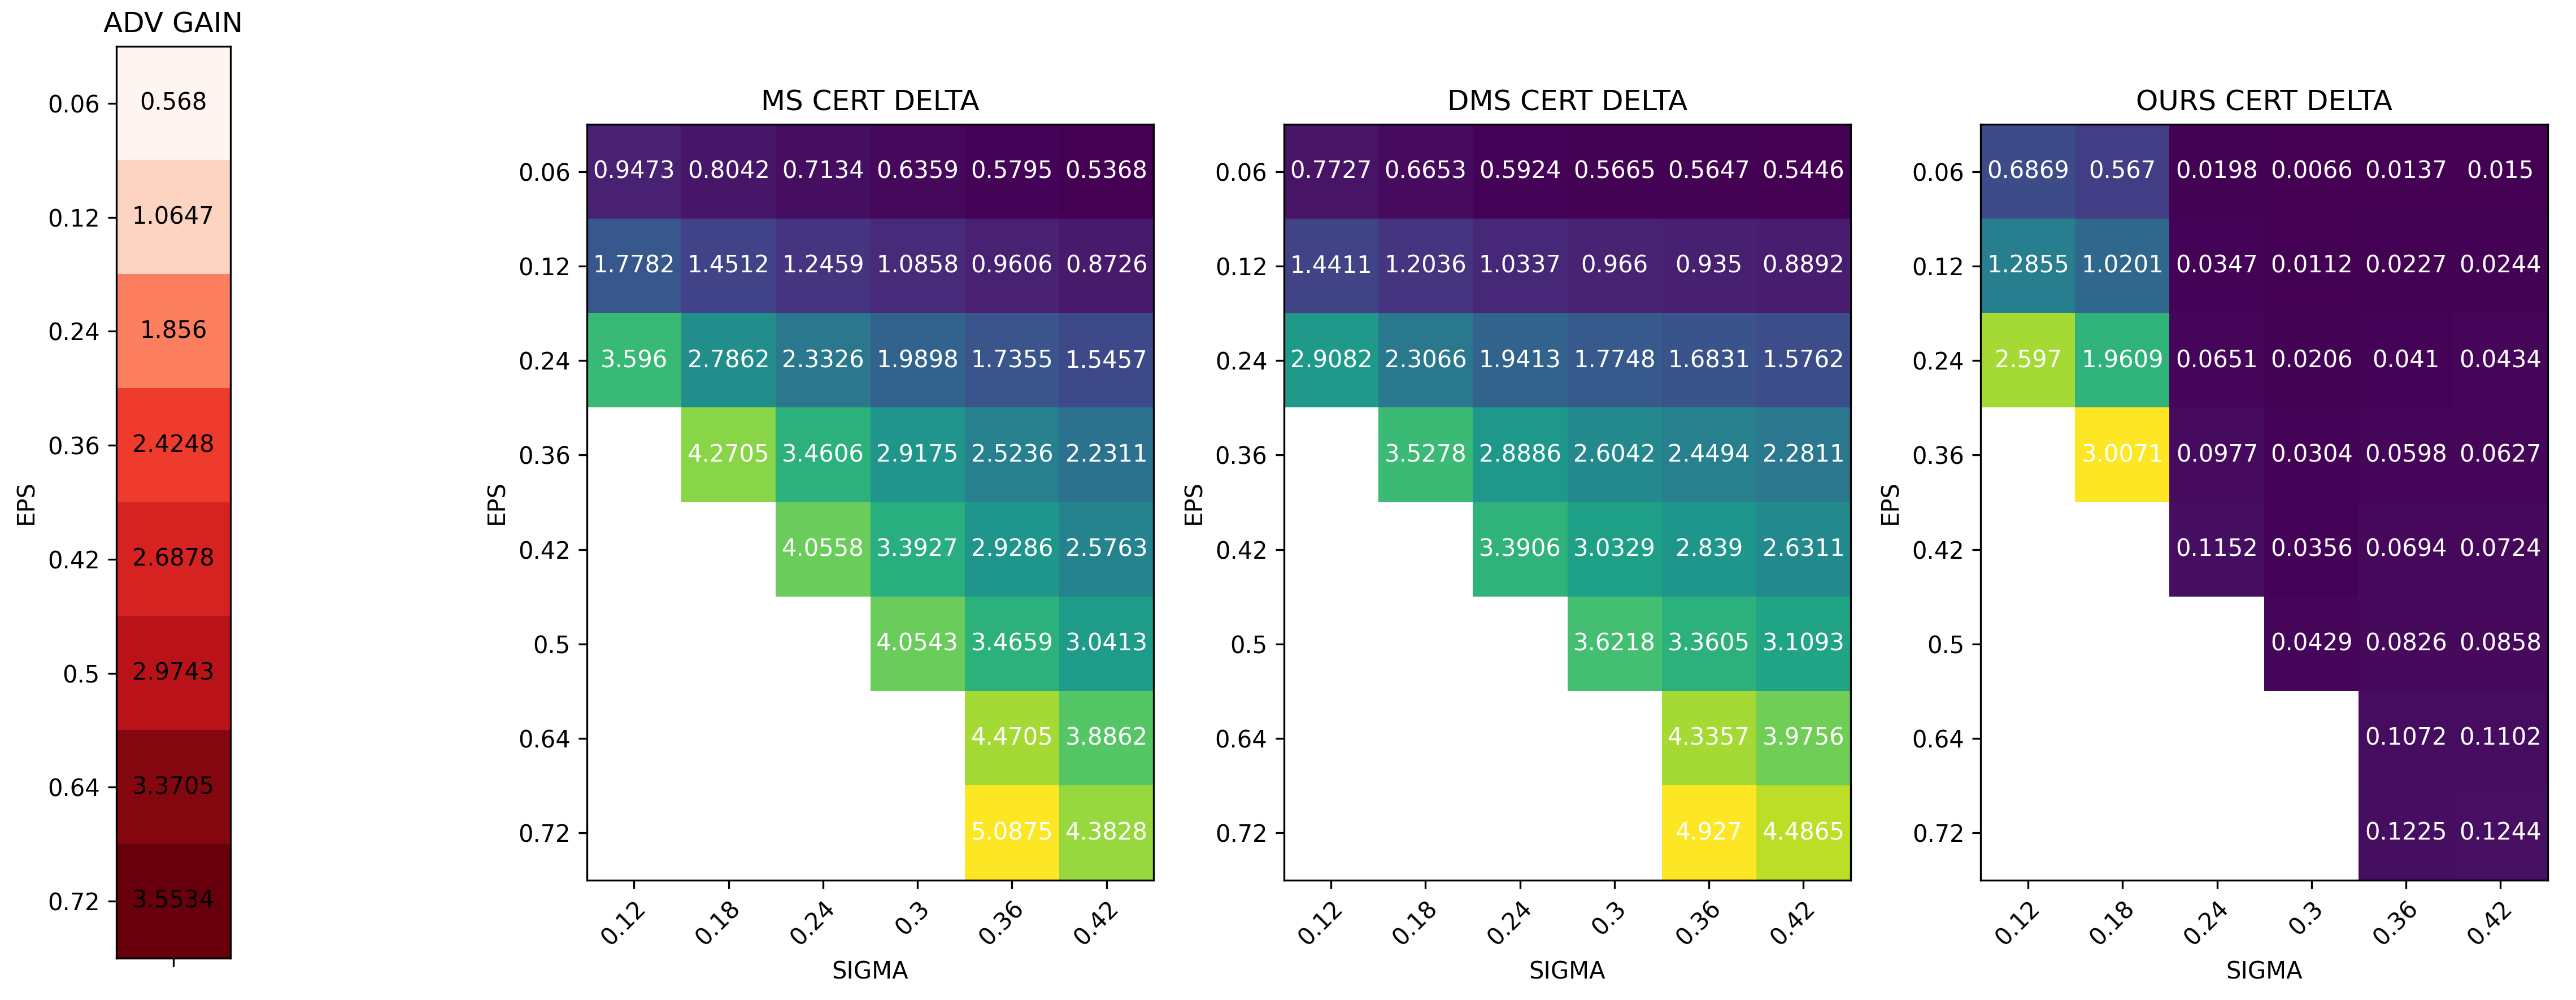}}
\caption{Certified Delta $\downarrow$}
\label{fig:heatmap_cdelta}
\end{center}
\end{figure*}

\subsection{Results for different datasets and IQA metric under defense}

TODO refer to tables

\begin{table*}[htb]
\caption{[absolute values table] The results. SPAQ dataset.}
\label{tab:results_clear_data}
\begin{center}
\begin{small}
\begin{tabular}{lcccccccccc}
\toprule
Method & \multicolumn{2}{c}{KonCept} &  \multicolumn{2}{c}{Hyper-IQA} & \multicolumn{2}{c}{CLIP-IQA+} & \multicolumn{2}{c}{DBCNN}  & \multicolumn{2}{c}{Topiq}  \\
 & SRCC $\uparrow$ & CD $\downarrow$ & SRCC $\uparrow$ & CD $\downarrow$ & SRCC $\uparrow$ & CD $\downarrow$ & SRCC $\uparrow$ & CD $\downarrow$ & SRCC $\uparrow$ & CD $\downarrow$ \\
\midrule
No-Defence & 0.8176 & $\infty$ & 0.8464 & $\infty$ & 0.8446 & $\infty$ & 0.8073 & $\infty$ & 0.8476 & $\infty$ \\
\midrule
MS (weak) & 0.6775 & 1.1582 & 0.6732 & 0.0090 & 0.7520 & 0.0185 & 0.7180 & 0.0039 & 0.7031 & 0.0096 \\
DMS (weak) & 0.7995 & 1.1002 & 0.8336 & 0.0144 & 0.8298 & 0.0207 & 0.7940 & 0.0101 & 0.8267 & 0.0142 \\
DMS-IQA (weak) & 0.7775 & 1.234 & 0.8144 & 0.0105 & 0.8764 & 0.0175 & 0.8736 & 0.0053 & 0.8672 & 0.0141 \\
\midrule
MS (strong) & 0.5364 & 4.8997 & 0.5633 & 0.0321 & 0.5766 & 0.0631 & 0.6436 & 0.0139 & 0.5721 & 0.0365 \\
DMS (strong) & 0.7942 & 5.0189 & 0.8169 & 0.0622 & 0.7893 & 0.0861 & 0.7788 & 0.0465 & 0.8068 & 0.0628 \\
DMS-IQA (strong) & 0.7611 & 5.1425 & 0.7877 & 0.0407 & 0.8593 & 0.0635 & 0.8638 & 0.0302 & 0.8733 & 0.0658 \\
\bottomrule
\end{tabular}
\end{small}
\end{center}
\end{table*}

\begin{table*}[htb]
\caption{[absolute values table] The results. CLIVE dataset. }
\label{tab:results_clear_data}
\begin{center}
\begin{small}
\begin{tabular}{lcccccccccc}
\toprule
Method & \multicolumn{2}{c}{KonCept} &  \multicolumn{2}{c}{Hyper-IQA} & \multicolumn{2}{c}{CLIP-IQA+} & \multicolumn{2}{c}{DBCNN}  & \multicolumn{2}{c}{Topiq}  \\
 & SRCC $\uparrow$ & CD $\downarrow$ & SRCC $\uparrow$ & CD $\downarrow$ & SRCC $\uparrow$ & CD $\downarrow$ & SRCC $\uparrow$ & CD $\downarrow$ & SRCC $\uparrow$ & CD $\downarrow$ \\
\midrule
No-Defence & 0.8346 & $\infty$ & 0.8390 & $\infty$ & 0.8791 & $\infty$ & 0.8468 & $\infty$ & 0.8878 & $\infty$ \\
\midrule
MS (weak) & 0.5931 & 1.0428 & 0.5238 & 0.0083 & 0.7651 & 0.0200 & 0.6255 & 0.0038 & 0.3244 & 0.0102 \\
DMS (weak) & 0.8068 & 0.886 & 0.7969 & 0.0146 & 0.7876 & 0.0209 & 0.7820 & 0.0117 & 0.8570 & 0.0134 \\
DMS-IQA (weak) & 0.8154 & 0.956 & 0.8401 & 0.0146 & 0.8175 & 0.0172 & 0.8271 & 0.0051 & 0.8812 & 0.0123 \\
\midrule
MS (strong) & 0.4792 & 4.577 & 0.3506 & 0.0301 & 0.5882 & 0.0744 & 0.6090 & 0.0133 & 0.0913 & 0.0383 \\
DMS (strong) & 0.7966 & 4.0435 & 0.7881 & 0.0640 & 0.7587 & 0.0871 &  0.7853 & 0.0533 & 0.8375 & 0.0599 \\
DMS-IQA (strong) & 0.7973 & 4.3854 & 0.836 & 0.0609 & 0.8076 & 0.0681 & 0.7861 & 0.0289 & 0.8739 & 0.0554 \\
\bottomrule
\end{tabular}
\end{small}
\end{center}
\end{table*}

\begin{table*}[htb]
\caption{[absolute values table] The results. KonIQ dataset. (or averaged across all datasets). or table for datasets averaged across all metrics. Weak use case: ($\sigma=0.12, \epsilon=0.06$), strong use case: ($\sigma=0.18, \epsilon=0.36$)}
\label{tab:results_clear_data}
\begin{center}
\begin{small}
\begin{tabular}{lcccccccccc}
\toprule
Method & \multicolumn{2}{c}{KonCept} &  \multicolumn{2}{c}{Hyper-IQA} & \multicolumn{2}{c}{CLIP-IQA+} & \multicolumn{2}{c}{DBCNN}  & \multicolumn{2}{c}{Topiq}  \\
 & SRCC $\uparrow$ & CD $\downarrow$ & SRCC $\uparrow$ & CD $\downarrow$ & SRCC $\uparrow$ & CD $\downarrow$ & SRCC $\uparrow$ & CD $\downarrow$ & SRCC $\uparrow$ & CD $\downarrow$ \\
\midrule
No-Defence & 0.8576 & $\infty$ & 0.9297 & $\infty$ & 0.8122 & $\infty$ & 0.8920 & $\infty$ & 0.9192 & $\infty$ \\
\midrule
MS (weak) & 0.5735 & 0.9473 & 0.6147 & 0.0113 & 0.6972 & 0.0207 & 0.6329 & 0.0042 & 0.5726 & 0.0102 \\
DMS (weak) & 0.7049 & 0.7727 & 0.8276 & 0.0124 & 0.7329 & 0.0205 & 0.7608 & 0.0106 & 0.8285 & 0.0122 \\
DMS-IQA (weak) & 0.8410 & 0.6869 & 0.8514 & 0.0091 & 0.7798 & 0.0114 & 0.7873 & 0.0027 & 0.8763 & 0.0093 \\
\midrule
MS (strong) & 0.4437 & 4.2705 & 0.5005 & 0.0409 & 0.5280 & 0.0797 & 0.5625 & 0.0153 & 0.4099 & 0.0400 \\
DMS (strong) & 0.6547 & 3.5278 & 0.7818 & 0.0557 & 0.7036 & 0.0878 & 0.7306 & 0.0492 & 0.7780 & 0.0560 \\
DMS-IQA (strong) & 0.8099 & 3.0071 & 0.8029 & 0.0370 & 0.7563 & 0.0535 & 0.7670 & 0.0136 & 0.8180 & 0.0403 \\
\bottomrule
\end{tabular}
\end{small}
\end{center}
\end{table*}

\subsection{Examples for usage smoothed IQA metric as a loss function}

This section provides images generated using the approach described in Section 6 (``Usage in the loss function''). TODO ref...
